# Supplementary material for: BenLLMEval: A Comprehensive Evaluation into the Potentials and Pitfalls of Large Language Models on Bengali NLP
Source: arXiv:2309.13173 source file (2024-03-19)
Supplement: Supplementary file 1 [file appendix_tables.tex]

\begin{figure*}[t]
\centering
\begin{subfigure}{.32\textwidth}
    \centering
    \includegraphics[scale=0.4]{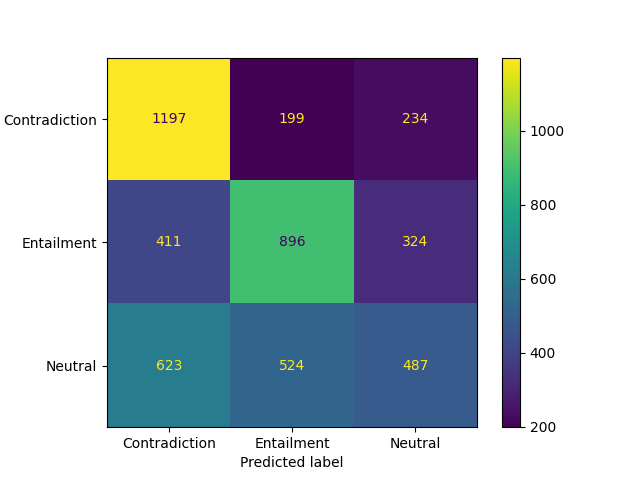}  
    \caption{GPT-3.5}
    \label{SUBFIGURE LABEL 1}
\end{subfigure}
\begin{subfigure}{.32\textwidth}
    \centering
    \includegraphics[scale=0.4]{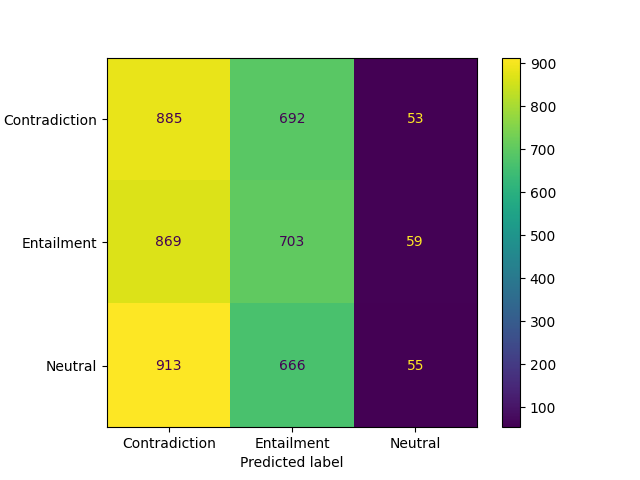}  
    \caption{Llama-2-13b-chat}
    \label{SUBFIGURE LABEL 2}
\end{subfigure}
\begin{subfigure}{.32\textwidth}
    \centering
    \includegraphics[scale=0.4]{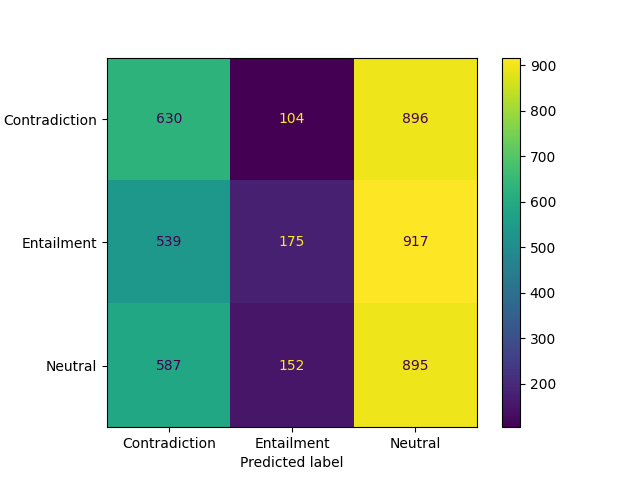}  
    \caption{Claude-2}
    \label{SUBFIGURE LABEL 3}
\end{subfigure}
\caption{Confusion matrices for different LLMs on the BNLI dataset for the NLI task. }
\label{FIGURE LABEL}
\end{figure*}

\subsection{Prompt Construction Details}
In the process of adapting datasets into prompts, we carefully analyzed the prompt templates in various LLM evaluation papers on English datasets \cite{laskar-etal-2023-systematic, qin2023chatgpt} and then explored several prompt variants in Bengali for each task to ascertain the optimal one. For example, at the beginning of the Soham News Article Classification task, our prompts did not feature class labels, which caused a pronounced failure in the accurate classification of news articles by all tested LLMs, markedly degrading their effectiveness. However, this situation improved considerably when we updated the prompts to integrate class labels, leading to a notable improvement in the models' capacity to correctly associate articles with their respective classes. Thus, experimenting with different variations of prompts to come up with the optimal one is a crucial step in our prompt design phase.

\subsection{In-depth Error Analysis}
\label{sec:error_analysis}
In this section, we discuss some interesting cases where GPT-3.5 failed to generate coherent responses given the input prompt. We discuss these cases in the following sections:

\subsection{Generative Tasks}
\label{sec:generative}

The error cases for generative tasks like abstractive summarization, question answering, and paraphrasing is discussed in this section. 

\subsection{Abstractive Summarizatoin}
\label{sec:as}

In the summarization task, we notice that GPT-3.5's responses are highly inconsistent. While GPT-3.5 occasionally recognizes the context and provides a good summary of the key points, it frequently misses these details in the reference text and overstuffs the response. One example can be demonstrated as follows: \\
\textbf{Prompt:} Please provide an one-sentence summary of the following Bangla text input. The input will be a long Bangla paragraph, the output should be a short Bangla paragraph summarizing only the vital information of the input text in one sentence. Please make sure that the output contains the most essential statistical data.
Note: Please do not provide anything other than the summarized Bangla output. \\
\textbf{Input:} \textbengali{মানসুর আব্বাস প্রধানমন্ত্রী বা তার প্রতিপক্ষ - কেউই আসলে ক্ষমতায় যাবার মতো নিরঙ্কুশ সংখ্যাগরিষ্ঠতা পাননি। আর এর মধ্যেই কিংমেকার হয়ে উঠেছে রাম (Raam) নামে একটি ইসলামপন্থী আরব দল (ইউনাইটেড আরব লিস্ট হিসেবেও দলটি পরিচিত)। এবারের নির্বাচনে পাঁচটি আসনে জয় পেয়েছে এ দলটি- যা মিস্টার নেতানিয়াহুকে ক্ষমতায় রাখা বা ক্ষমতা থেকে বিদায় করে দিতে ভূমিকা রাখার সুযোগ করে দিয়েছে। বিবিসি বাংলায় আরও পড়ুন: ফিলিস্তিনি-ইসরায়েলি সংঘাতের মূলে যে দশটি প্রশ্ন ইসরায়েলকে ইহুদি রাষ্ট্র ঘোষণার প্রতিক্রিয়া কী হবে? ইসরায়েলের কাছে আরবরা কেন পরাজিত হয়েছিল? ২০১৯ সাল থেকে নেতৃত্ব দিচ্ছেন মানসুর আব্বাস রাম: বিস্ময়কর কিংমেকার রক্ষণশীল মুসলিম মানসুর আব্বাসের নেতৃত্বে রাম দলটি মূলত ফিলিস্তিনের গাজা শাসন করা হামাসের ধর্মীয় ভাবধারায় গড়ে ওঠা একটি ইসলামপন্থী দল। ১৯৯৬ সালে প্রতিষ্ঠিত এই দলটি শুরু থেকে ইসরায়েলের পার্লামেন্ট আসন পেয়ে আসছে। যদিও ২০০৯ সালের নির্বাচনে অংশ নেয়ার ক্ষেত্রে তাদের ওপর নিষেধাজ্ঞা দিয়েছিলো দেশটির নির্বাচনী কর্তৃপক্ষ। পরে সুপ্রিম কোর্ট ওই নিষেধাজ্ঞা বাতিল করে দেয়। ২০২০ সালে ইসরায়েলের আরব রাজনৈতিক দলগুলোর জোট- জয়েন্ট আরব লিস্টের অংশ ছিলো যারা নজিরবিহীন ভাবে পনেরটি সিট পেয়েছে পার্লামেন্টে। তবে একাই নির্বাচনে লড়ার জন্য চলতি বছরের ২৮শে জানুয়ারি ওই জোট ছেড়ে আসে রাম। আরব সম্প্রদায়ের সামগ্রিক দরকষাকষির ক্ষমতাকে হুমকির মুখে ফেললেও এ সিদ্ধান্ত দলটির 'কিংমেকার' হয়ে ওঠার পথও তৈরি করে দিয়েছে। নির্বাচনে ভোট দিচ্ছেন এক ইসরায়েলি-আরব নারী দলটির পেছনে থাকা ব্যক্তি ৪৬ বছর বয়সী মানসুর আব্বাস হলেন দলটির মূল ব্যক্তি। ইসরায়েলের রাজনৈতিক ইতিহাসের গুরুত্বপূর্ণ সময়টিতে তিনি এখন রাজনীতির কেন্দ্রে রয়েছেন। জেরুজালেমের হিব্রু বিশ্ববিদ্যালয় থেকে পাশ করা দন্ত চিকিৎসক তিনি। যদিও পরে হাইফা বিশ্ববিদ্যালয় থেকে রাষ্ট্রবিজ্ঞানে মাস্টার্স ডিগ্রি লাভ করেন। ২০১৯ সালে তিনি ইউনাইটেড আরব লিস্টের নেতা মনোনীত হন এবং ওই জোটের অংশ হিসেবে পার্লামেন্টেও নির্বাচিত হন। অবশ্য বেনিয়ামিন নেতানিয়াহু ও তার লিকুদ পার্টির সাথে যোগাযোগ বাড়ানোর চেষ্টা করতে গিয়ে তিনি দলের মধ্যে বিভক্তিও তৈরি করেন। ইসরায়েলে আরব রাজনীতি ইসরায়েলের প্রায় নব্বই লাখ মানুষের মধ্যে উনিশ লাখের মতো আরব আছেন যারা ১৯৪৮ সালে ইসরায়েলের সীমানায় থেকে গিয়েছিলেন। ওই প্রায় সাড়ে সাত লাখ ফিলিস্তিনি তাদের বাড়িঘর ছেড়ে পালিয়েছিলো অথবা তাদের বহিষ্কার করা হয়েছিলো। যদিও ইসরায়েলের নাগরিক এমন অনেক আরব নিজেদের ফিলিস্তিনি বা ইসরায়েলি ফিলিস্তিনি হিসেবে পরিচিত হতে পছন্দ করেন আর অন্যরা নিজেদের ইসরায়েলি আরব হিসেবে উল্লেখ করে থাকে। ইসরায়েলের আরবদের বেশিরভাগই সুন্নি মতাদর্শে বিশ্বাসী আর দ্বিতীয় বড় অংশটি খ্রিস্টান। ইসরায়েলের দশ শতাংশ মুসলিম আরব বেদুইন গোত্র থেকে আসা। ১৯৪৯ সালের নির্বাচনে তারা অংশ নিয়েছিলো। আরব রাজনৈতিক দলগুলো দেশটিতে আরবদের সমান অধিকারের পক্ষে সোচ্চার ভূমিকা পালন করে এবং একই সাথে ফিলিস্তিনের প্রতিও তাদের সমর্থন আছে। বেনজামিন নেতানিয়াহু এখন রাম কোনো জোটে যাবে? গত বছর মিস্টার নেতানিয়াহুর প্রতিপক্ষ বেনি গান্টজ আরব দলগুলোর সাথে জোট করে সরকার গঠনের বিষয়টি প্রত্যাখ্যান করেছিলেন। এর আগে নেতানিয়াহু নিজেও রামের সাথে জোটের সম্ভাবনা উড়িয়ে দিয়েছিলেন। যদিও প্রচারণায় তার সুর ছিলো নরম। এখন যদি তারা একটি জোট করতে পারেন তাহলে মিস্টার নেতানিয়াহু ও মিস্টার আব্বাস- দুজনেই লাভবান হবেন। যদিও সংবাদদাতারা বলছেন, নেতানিয়াহুর অন্য শরীকদের সাথে তারা কিভাবে একযোগে কাজ করবেন তা এখনো পরিষ্কার নয়। জেরুজালেমে বিবিসি সংবাদদাতা অবশ্য বলছেন কোয়ালিশনে না থেকেও মিস্টার নেতানিয়াহুকে সমর্থন দেয়ার চুক্তি করতে পারে রাম। কিন্তু চুক্তি বা সমঝোতা যাই হোক- মিস্টার আব্বাস এখন নিশ্চিত যে দরকষাকষির সুযোগ তার হাতে। তিনি বলেছেন ইসরায়েলের আরব জনগোষ্ঠীর জন্য সেরা সিদ্ধান্তটিই তিনি নেবেন। যদিও অনেকেই এখনো এ নিয়ে নিশ্চিত নন। জেরুজালেম অধিকার কর্মী ইতাফ আওয়াদ বলছেন, লিকুদ ও রাম দলের জোট ফিলিস্তিনিদের জন্য ভালো হবে না।} \\
\textbf{Expected Response:} \textbengali{গত দু বছরের মধ্যে চতুর্থবারের মতো একই সমস্যা হচ্ছে ইসরায়েলে- নির্বাচনের পর সংখ্যাগরিষ্ঠতা পেয়েও ক্ষমতায় থাকার জন্য প্রয়োজনীয় আসনের জন্য হাহাকার করতে হচ্ছে প্রধানমন্ত্রী বেনিয়ামিন নেতানিয়াহুকে।}\\
\textbf{GPT-3.5 Response:} \textbengali{ মানসুর আব্বাস নেতৃত্বের রাম দল ইসরায়েলের পার্লামেন্টে পাঁচটি আসন জিতেছে এবং এদের কিংমেকার হয়ে উঠার পথ তৈরি করেছে, তিনি ইউনাইটেড আরব লিস্টের নেতা হিসেবে পরিচিত এবং ইসরায়েলে আরব রাজনীতি প্রায় নব্বই লাখ মানুষের মধ্যে উনিশ লাখের মতো আরব আছেন যারা ১৯৪৮ সালে ইসরায়েলের সীমানায় থেকে গিয়েছিলেন।}\\
In the aforementioned example, GPT-3.5 fails to highlight the most crucial information from the input and saturates the output with superfluous texts.

\subsubsection{Question Answering}
\label{sec:QA}
In the Question Answering task, GPT-3.5 is given instructions to provide responses based on the given context. However, there are instances where GPT-3.5 deviates from the context and attempts to answer using information from its general knowledge, resulting in a mismatch with the gold label. While this problem occurred only in a limited number of cases, the authors were unable to independently verify the accuracy of the responses in these instances, leading to their classification as incorrect answers.\\
\textbf{Prompt:} Please provide an answer to the input Bangla question based on the given Bangla context. The input will contain a Bangla question followed by a context. The output should be the answer in Bangla based on the context. Note: Please do not provide anything other than the Bangla answer to the question.\\
\textbf{Context:} \textbengali {নেপালের রাজধানী কাঠমুন্ডুর উপত্যকায় প্রাপ্ত নিওলিথিক যুগের বেশকিছু উপাদান এটিই নির্দেশ করে যে হিমালয়ান অঞ্চলে প্রায় ৯০০০ বছর থেকে মানুষ বসবাস করছে। এটি প্রতিষ্ঠিত যে প্রায় ২৫০০ বছর পূর্বে নেপালে তিব্বতী-বার্মীয় জনগোষ্ঠীর বসবাস ছিল। ১৫০০ খৃস্টপূর্বাব্দে ইন্দো ইরানীয় বা আর্য জাতিগোষ্ঠী এই হিমালয়ান উপত্যকায় প্রবেশ করে। ১০০০ খৃস্টপূর্বাব্দের দিকে এই অঞ্চলটিতে বিভিন্ন গোষ্ঠীর জন্য স্বতন্ত্র রাজ্য ও কনফেডারেশন গড়ে উঠে। এরকমই একটি কনফেডারেশন ছিল সাকিয়া যার একসময়কার রাজা ছিলেন সিদ্ধার্থ গৌতম (৫৬৩-৪৮৩ খৃস্টাপূর্বাব্দ) যিনি গৌতম বুদ্ধ বা শুধু বুদ্ধ নামেই পরিচিত। তিনি পবিত্র ও সাধনাময় জীবনযাপনের জন্য তার রাজত্ব ত্যাগ করেছিলেন। ২৫০ খৃস্টপূর্বাব্দে এই অঞ্চলটি উত্তর ভারতের মৌর্য সম্রাজ্যের (Mauryan) অধীনে আসে এবং পরবর্তীতে ৪র্থ শতাব্দীতে এটি গুপ্ত সম্রাজ্যের অধীনে একটি পুতুল রাষ্ট্রে পরিণত হয়। পঞ্চম শতাব্দীর শেষ হতে শুরু করে পরবর্তী বেশ কিছুটা সময় শাসন করে একদল শাসক যারা সাধারণভাবে লিচ্ছবি (Licchavis) নামে পরিচিত। লিচ্ছভি সাম্রাজ্যের (Licchavi) পতন ঘটে অষ্টম শতাব্দীতে এবং এরই সাথে শুরু হয় নেওয়ারি (Newari) যুগের। ৮৭৯ সালে নেওয়ারিদের রাজত্ব শুরু হলেও সমগ্র রাষ্ট্রের উপর তাদের নিয়ন্ত্রণ অনেকটাই অনিশ্চিত ছিল। একাদশ শতাব্দীর শেষ ভাগে নেপালের দক্ষিণাংশ দক্ষিণ ভারতের চালুক্য সাম্রাজ্যের (Chalukaya) অধীনে আসে। চালুক্যদের রাজত্বকালে নেপালের ধর্মে ব্যাপক পরিবর্তন আসে কারণ সব রাজাই হিন্দু ধর্মের পৃ্ষ্ঠপোষকতা করতেন এবং বৌদ্ধ ধর্মের প্রসারের বিপরীতে হিন্দু ধর্মের প্রচারে অবদান রাখেন।}\\
\textbf{Question:} \textbengali{নেপাল কি একটি সার্বভৌম দেশ ?}\\
\textbf{Expected Response: } No Answer.\\
\textbf{GPT-3.5 Response: } \textbengali{হ্যাঁ, নেপাল একটি সার্বভৌম দেশ।}\\
In this particular instance, GPT-3.5 provides responses that go beyond the scope of the given context, as the context itself lacks the necessary information to yield the correct answer. Consequently, this deviation from the context leads to a mismatch with the gold label, ultimately resulting in an incorrect response.

\subsubsection{Paraphrasing}
\label{sec:paraphrase}
In some instances, GPT-3.5 generates paraphrase that completely changes the meaning of the input sentences. For example: \\
\textbf{Input: } \textbengali{আগুনে কোনও হতাহতের খবর পাওয়া যায়নি।} [No injury was reported because of the fire] \\
\textbf{Expected Responses: } [\textbengali{'অগ্নিকাণ্ডে উল্লেখযোগ্য কোন ক্ষয়ক্ষতি হয়নি।', 'অগ্নিকাণ্ডে উল্লেখযোগ্য কোন ক্ষয়ক্ষতি হয়নি।', 'এই অগ্নিকাণ্ডে হতাহতের কোনও খবর মেলেনি।', 'এই অগ্নিকাণ্ডে হতাহতের কোনো খবর পাওয়া যায়নি।', 'অগ্নিকাণ্ডে হতাহতের কোনো খবর পাওয়া যায়নি।', 'অগ্নিকাণ্ডে কারও হতাহতের খবর পাওয়া যায়নি।'}]\\
\textbf{GPT-3.5 Response:} \textbengali{কোন আপত্তিকর ঘটনা না হওয়ায় আগুনের সম্পর্কে কোন খবর পাওয়া যায়নি।} [There was no news about the fire as there was no untoward incident.]
This is a matter of concern and presents additional evidence that GPT-3.5 is not currently suitable for serving as a universal problem solver in the Bangla language.

\subsection{Classification Tasks}
\label{sec:txtcls}
In this section, we discuss the error cases in the other three tasks that we consider: Natural Language Inference (NLI), Text Classification, and Sentiment Analysis. 

\subsubsection{Natural Language Inference}
\label{sec:nli}
The confusion matrix obtained by evaluating GPT-3.5 for the NLI task is demonstrated in Figure \ref{FIGURE LABEL}. The matrix reveals that GPT-3.5 demonstrates high accuracy in predicting the \textit{Contradiction} and \textit{Entailment} labels, but encounters significant challenges in accurately predicting the \textit{Neutral} labels. Approximately 49\% of the misclassifications arise when attempting to predict the \textit{Neutral} class. A thorough manual examination uncovers that GPT-3.5 often exhibits bias towards expressing a particular opinion polarity (\textit{Contradiction, Entailment}) when dealing with logical relationships in Bangla, and it fails to appropriately recognize and convey neutrality even in cases where it is evident.

% \begin{figure}[h]
% \centering
% \includegraphics[scale = 0.53]{figures/foo.png}
% \caption{Confusion matrix obtained by evaluating GPT-3.5 for the NLI task on BNLI dataset}
% \label{fig:conf_nli}
% \end{figure}

\textbf{Prompt:} Please determine the logical relationship between the given hypothesis and premise. The input will consist of two sentences written in the Bangla language. The first sentence represents the premise, while the second sentence represents the hypothesis.  Your task is to determine whether the hypothesis is false (contradiction), true (entailment), or inconclusive (neutral) given the premise. Please output a number indicating the logical relationship between them: 0 for false (contradiction), true (entailment), and 2 for inconclusive (neutral) for neutrality. 
Note: Please avoid providing any additional information beyond the logical relationship. \\
\textbf{Premise:} \textbengali{ঠিক আছে, যেখানে দুই-তিনটা বিমান এক সপ্তাহে এসে পৌছেছে এবং আমি জানতাম না তারা কোথায় যাচ্ছে।} \\
\textbf{Hypothesis:} \textbengali{প্রতি সপ্তাহে একটিরও বেশি বিমান আসে।}\\
\textbf{Expected Response: }1 (Entailment)\\
\textbf{GPT-3.5 Response: }2 (Neutral) 

\subsubsection{Transliteration}
\label{sec:trans}
A deeper look into the cases where LLMs fail yields the following observations:

\vspace{-2pt} 
\textbf{(i) Intricate pronunciation rules in Bengali pose challenges in transliteration.} Bengali, being a language rich in nuances, possesses distinct rules for pronunciation and spelling. In Bengali, the same letter may produce different sounds when used in different words. All LLMs encounter significant challenges in scenarios where specific rules govern the pronunciation of a particular letter. For instance, the Latin lexicon `\textit{andre}' is pronounced as `\text{\bengalifont{আঁদ্রে}}' in Bengali (similar to \textit{`addre'} in English). The \textit{`n'} letter of the lexicon `\textit{andre}' is silent in Bengali and instead represented as `\text{\bengalifont{ঁ}}', which creates a nasal sound, whereas even the response of GPT-3.5 (which is the best-performing LLM in this task) is `\text{\bengalifont{আন্দ্রে}}', which includes an `\textit{n}' sound. Such unconventional cases represent the primary reasons for LLMs to struggle while transliterating lexicons from Latin to Bengali.

\vspace{2pt} 
\textbf{(ii) Difficulty in transliterating lexicons that closely resemble English words.} For instance, when encountering the term `\textit{cador}', which bears a strong resemblance to the English word \textit{cadre}', GPT-3.5 mistakenly transliterates it as `\text{\bengalifont{ক্যাডর}}', a transliteration that shares a similar pronunciation to `\textit{cadre}'. However, the correct gold label for this particular example is `\text{\bengalifont{চাদর}}'. Such instances of erroneous substitution lead to an increase in CER.  

\vspace{-2pt} 
\textbf{(iii) Transliteration of outdated pronunciations.} Languages continuously undergo changes based on their usage by individuals. In the Dakshina dataset, certain gold labels are annotated with outdated pronunciations. While LLMs correctly transliterate various lexicons into more contemporary pronunciations, many such instances in the Dakshina dataset are considered incorrect transliterations due to outdated gold labels. For instance, the term `\textit{ssoshur}' is transliterated as `\text{\bengalifont{শ্বশুর}}' by GPT-3.5, which represents an accurate contemporary transliteration. Nevertheless, the gold label for this example is given as `\text{\bengalifont{শশুর}}'. Such cases 
%predominantly 
result in 90\% of the substitution errors in GPT-3.5. 

\textbf{Full Sentence Transliteration:} As seen from table \ref{tab:translit_eval}, the zero-shot GPT-3.5 on full sentence transliteration surpasses all the SOTA models except one (i.e., \textit{Noisy Channel}). Meanwhile, Claude-2 achieves comparable performance with the prior models. The error patterns encountered in full-sentence transliteration largely align with those observed in single-word transliteration, with the addition of the following error case:

\textbf{ (i) Code-mixing creates a stumbling block for GPT-3.5.} While transitioning %from Bangla-English-Bangla 
between vocabulary words, LLMs demonstrate a tendency to make mistakes. For instance, the following sentence `\textit{Amake to tomra \textcolor{red}{mute} kore rekhechile}' contains an occurrence of code-mixing with the English word `\textit{mute}'. GPT-3.5 misidentifies it as a Bengali word and transliterates the sentence as `\text{\bengalifont{আমাকে তো তোমরা \textcolor{red}{মুটে} করে রেখেছিলে}}', whereas the accurate transliteration of the word `\textit{mute}' should be `\text{\bengalifont{মিউট}}' instead of `\text{\bengalifont{মুটে}}'. Such cases contribute to substitution errors in full-sentence transliteration.

\subsubsection{News Article Classification}
\label{sec:newscls}
Our experimental results show that GPT-3.5 misclassified the category \textit{kolkata} the most, failing to generate the correct response in 503 of the test set's 569 examples (88.4\%). The subsequent category with the highest frequency of misclassification is \textit{national}. GPT-3.5 was unable to accurately classify this particular category in 95 out of 175 instances, representing a misclassification rate of 54.20\%. On the other hand, GPT-3.5 effectively identified the category labeled as \textit{entertainment} in 110 out of 130 occurrences, resulting in a success rate of 92.30\%.

\subsubsection{Sentiment Analysis}
\label{sec:senti}
The examples listed in Table \ref{tab:Sentiment_error}, illustrate the error cases where GPT-3.5 misclassifies the sentiment of the given input. The first seven examples are from the IndicSentiment test set and the rest of the examples are from the SentNoB dataset. Notably, the \textit{positive} class exhibits the most frequent misclassification in both test sets, suggesting that GPT-3.5 still has a considerable way to go toward attaining a complete understanding of the Bangla language. In the instances where the class is \textit{neutral}, the examples are mostly simple statements with no sentiment word associated with them (table entries 11, and 12), yet GPT-3.5 classified them as either \textit{negative} or \textit{positive}. Furthermore, GPT-3.5 demonstrates difficulties in capturing challenging Bangla sentiment words, i.e., \textbengali{অমায়িক} (\textit{Accommodating} in English), \textbengali{সুবিধা} (\textit{Advantage} in English), \textbengali{আপসহীন} (\textit{Uncompromising} in English) etc (example 2, 8, 13 in Table \ref{tab:Sentiment_error}).

\subsection{Unexpected, out of range response}
\label{sec:outres}
In the tasks of text classification and sentiment analysis, the prompts are designed to include the target classes in order to identify any unexpected or non-class responses. Based on our experimental findings, we observe that the outputs generated by GPT-3.5 exhibit outcomes that deviate from the expected range of outputs. \\
\textbf{\underline{News Article Classification.}} \\
\textbf{Prompt:} For the Bengali news article given in the input, identify the appropriate section title for the article from the following classes: kolkata, state, sports, national, entertainment, international. Note: Do not output any unnecessary words other than just the section title. The response should be in English language and should be one word.
Input : \textbengali{১০০ দিনের কাজের প্রকল্পের সাফল্য দেখতে রাজ্যে আসছেন কেন্দ্রের প্রতিনিধি। সঙ্গে ১০টি রাজ্যের প্রতিনিধিও। ৯ থেকে ১২ জানুয়ারির মধ্যে পাঁচটি জেলায় রাজ্যের ‘উদ্ভাবনী কাজে’র সাফল্য দেখবেন তাঁরা। ঘটনাচক্রে, পঞ্চায়েত নির্বাচনের আগে এই সফর হতে চলেছে। ফলে প্রশাসনের একাংশের মতে, এই সফর ভোটের আগে শাসকদলের কাছে বড় প্রাপ্তি হতে পারে। বিশেষত, রাজ্যগুলির মধ্যে অধিকাংশই যখন বিজেপি অথবা বিজেপি’র সহযোগী দলের সরকার পরিচালিত। ‘ইন্টার স্টেট এক্সচেঞ্জ প্রোগ্রামে’র আওতায় প্রতি বছর একটি বা দু’টি রাজ্যকে বেছে নেওয়া হয়। চলতি বছরে এ রাজ্যকে বেছে নিয়েছে কেন্দ্র। কেন্দ্রীয় সরকারের যুগ্মসচিব (এনআরইজিএ) অপরাজিতা সারেঙ্গির নেতৃত্বে ১১ জন পদস্থ আধিকারিক আসবেন। থাকবেন ১০টি রাজ্য থেকে পাঁচজন করে সরকারি প্রতিনিধি। রাজ্যগুলির মধ্যে রয়েছে তামিলনাড়ু, অন্ধ্র, তেলঙ্গনা, কর্নাটক, ও়ড়িশা, বিহার, হিমাচলপ্রদেশ, ছত্তীসগঢ় এবং মধ্যপ্রদেশ। জম্মু ও কাশ্মীর প্রতিনিধি পাঠাবে কি না, তার নিশ্চয়তা মেলেনি। পাঁচটি দলে ভাগ করে প্রতিনিধিদের নিয়ে যাওয়া হবে পশ্চিম বর্ধমান, বাঁকুড়া, পুরুলিয়া, ঝাড়গ্রাম এবং বীরভূমে। ১০০ দিনের কাজের প্রকল্পের আওতায় শুকিয়ে যাওয়া ঝরনায় বিকল্প উপায়ে জলের জোগান ফিরিয়ে আনা, ফ্লাই অ্যাশের ইট তৈরি, পুরুলিয়ার মাটিতে বেদানার ফলন, মাটির চরিত্র ভিন্ন হলেও আরবের খেজুর চাষ, লাতিন আমেরিকা এবং দক্ষিণ পূর্ব এশিয়ার জনপ্রিয় ড্রাগন ফ্রুটের চাষ, বৃক্ষপাট্টা দিয়ে গাছ বাঁচানো-সহ বিভিন্ন কাজ প্রতিনিধিদলের সামনে তুলে ধরা হবে। এই অভিজ্ঞতা ভবিষ্যতে কীভাবে ছড়িয়ে দেওয়া যায়, তা দেখবেন তাঁরা। ৯ জানুয়ারি দুর্গাপুরে প্রতিনিধিদলের সঙ্গে বৈঠক করবেন রাজ্যের পঞ্চায়েতমন্ত্রী সুব্রত মুখোপাধ্যায়, মুখ্যসচিব মলয় দে-সহ দফতরের আধিকারিকেরা। সফরের শেষেও বৈঠক হবে। রাজ্যের এনআরইজিএ কমিশনার দিব্যেন্দু সরকারের কথায়, ‘আমাদের স্লোগান আজকের মজুরি, আগামীর জীবিকা। শুধু মাটি কাটা নয়, সদিচ্ছা থাকলে এই প্রকল্পের আওতায় যে ভিন্ন ধরনের কাজ করা সম্ভব, প্রতিনিধিদের তা দেখানো হবে’।} \\
\textbf{Expected Response:} State \\
\textbf{GPT-3.5 Response:} Development \\
Our study reveals that GPT-3.5, in particular, generated the word \textit{Development}, which deviates from the prompted range of responses. The generated output is considered out of range as the prompt specifically instructs the model to produce text within the given categories of \textit{kolkata}, \textit{state}, \textit{sports}, \textit{national}, \textit{entertainment}, and \textit{international}. In addition, the results of our experiment indicate that GPT-3.5 produced 12 classes that are outside the target class range, thus demonstrating the model's inability to comply with the specified instructions for this specific task. \\
\textbf{\underline{Sentiment Analysis.}} \\
\textbf{Prompt:} For the given Input, is the sentiment in the input positive or negative?
Note: Please do not output anything other than the sentiment. Exclude any word like, Sentiment in the response. \\
Input : \textbengali{স্ট্যান্ড-এ রয়েছে লেভেল ইন্ডিকেটর যা বিল্ট-ইন বাবল ভিউ লেভেল এবং থ্রি-ওয়ে হেড যা ৩৬০ ডিগ্রি ঘোরানো যায়।} \\
\textbf{Expected Response:} Positive \\
\textbf{GPT-3.5 Response:} Neutral \\
In this instance, although we explicitly prompted GPT-3.5 to generate output that is either positive or negative, it produced a response that falls outside of the designated range, i.e., \textit{Neutral}. This observation implies that the model may possess certain inherent biases towards sentiment classification among the three widely used categories, namely \textit{positive}, \textit{negative}, and \textit{neutral}. 

%%%%%%%%%%%%%%%%%%%%%%%%%%%%%%%%%%%%%%%%%%%%%%%%%%%%%%%%%%%%
\begin{table*}[htbp!]
\centering
\scriptsize
\begin{tabular}{{p{.10\linewidth}p{.12\linewidth}p{.40\linewidth}p{.15\linewidth}p{.15\linewidth}}}
\hline
\textbf{Dataset} & \textbf{Task Type} & \textbf{Prompt} & \textbf{GPT-3.5 Response} & \textbf{Gold Label}\\
\hline
XL-Sum & Text Summarization  & Please provide an one-sentence summary of the following Bangla text input. The input will be a long Bangla paragraph, the output should be a short Bangla paragraph summarizing only the vital information of the input text in one sentence. Please make sure that the output contains the most essential statistical data.
Note: Please do not provide anything other than the summarized Bangla output. [INPUT: \textbengali{ঢাকার ইস্ট ওয়েস্ট বিশ্ববিদ্যালয় চত্বরে কাঁদানে গ্যাস এরপর বিশ্ববিদ্যালয় কর্তৃপক্ষ অনির্দিষ্টকালের জন্য বিশ্ববিদ্যালয় বন্ধ ঘোষণা করে। বিশ্ববিদ্যালয়ের একজন কর্মকর্তা নিশ্চিত করেছেন, ছাত্র-ছাত্রীদের এসএমএস করে সিদ্ধান্ত জানানো হচ্ছে। ওদিকে বাড্ডা এলাকায় ইস্ট ওয়েস্ট বিশ্ববিদ্যালয়ও দুদিনের জন্য বন্ধ ঘোষণা করা হয়েছে। বিশ্ববিদ্যালয়ের ওয়েবসাইটে এক ঘোষণায় বলা হয়েছে, অনিবার্য কারণে আগামি ৭ ও ৮ অগাস্ট বিশ্ববিদ্যালয় বন্ধ থাকবে। সকালের দিকে এই বিশ্ববিদ্যালয়ের ছাত্রদের সাথে পুলিশ এবং ছাত্রলীগের সংঘর্ষ হয়। আরও পড়ুন: জিগাতলা-সায়েন্স ল্যাব 'ঠান্ডা', অশান্ত বাড্ডা আইসিটি আইনে মামলায় শহীদুল আলম ৭ দিনের রিমান্ডে জানা গেছে, সেখানে সরকারি দলের অঙ্গ সংগঠন ছাত্রলীগের বেশ কিছু সদস্য সকাল ১০টার দিকে ছাত্র-ছাত্রীদের ক্যাম্পাস ঢুকতে বাধা দিলে সংঘর্ষ শুরু হয়। বিশ্ববিদ্যালয়ের জেনেটিক ইঞ্জিনিয়ারিং বিভাগের ছাত্র হৃদয় ইসলাম বিবিসিকে বলেছেন, ছাত্রলীগের ছেলেরা বেশ কিছু শিক্ষার্থীকে মারধর করে। ভাঙচুর করে। পরে পুলিশ বেশ কয়েক দফা কাঁদানে গ্যাস ছোঁড়ে। বাস চাপায় দুজন শিক্ষার্থীর মৃত্যু কেন্দ্র করে সপ্তাহখানেক ধরে স্কুলের ছাত্র-ছাত্রীরা যে বিক্ষুব্ধ আন্দোলন করছিলো - তাতে রোববার থেকে বিশ্ববিদ্যালয়ের ছাত্রদেরও যোগ দিতে দেখা যায়। আজ (সোমবার) রাস্তায় স্কুলের ছাত্র-ছাত্রীদের দেখা না গেলেও, কয়েকটি বিশ্ববিদ্যালয়ের শিক্ষার্থীরা বিক্ষোভ মিছিল বের করার চেষ্টা করে। নিরাপদ সড়ক: নর্থ সাউথ ও ইস্ট-ওয়েস্ট বিশ্ববিদ্যালয় বন্ধ ঘোষণা ]} & \textbengali{ঢাকার ইস্ট ওয়েস্ট বিশ্ববিদ্যালয় চত্বরে গ্যাস কাঁদানের পর অনির্দিষ্টকালের জন্য বন্ধ ঘোষণা করা হয়েছে, বাড্ডা এলাকায় ইস্ট ওয়েস্ট বিশ্ববিদ্যালয়ও দুদিনের জন্য বন্ধ ঘোষণা করা হয়েছে।} & \textbengali{সোমবার দুপুরের দিকে ঢাকার বসুন্ধরা এলাকায় নিরাপদ সড়ক ইস্যুতে বিক্ষোভ মিছিল বের করা নিয়ে নর্থ-সাউথ বিশ্ববিদ্যালয়ের ছাত্রদের সাথে পুলিশের সংঘর্ষ হয়। ছাত্রদের ছত্রভঙ্গ করতে পুলিশ সেসময় কাঁদানে গ্যাস ব্যবহার করে।} \\
\hline
SQuAD\_Bangla  & Question Answering  & Please provide an answer to the input Bangla question based on the given Bangla context. The input will contain a Bangla question followed by a context. The output should be the answer in Bangla based on the context. Note: Please do not provide anything other than the Bangla answer to the question.  [CONTEXT: \textbengali{অ্যাপল ইনকর্পোরেটেড এর সদর দপ্তর ক্যালির্ফোনিয়ার মধ্য সিলিকন ভ্যালীতে অবস্থিত। ৮৫০,০০ বর্গ ফিট জায়গাতে ৬টি বিল্ডিংয়ে অ্যাপলের বর্তমান সদর ১৯৯৩ সালে থেকে অবস্থান করছে।]}  [QUESTION: \textbengali{অ্যাপল ইনকর্পোরেটেডের সদর দপ্তর কোথায় ?]} & \textbengali{অ্যাপল ইনকর্পোরেটেড এর সদর দপ্তর ক্যালির্ফোনিয়ার মধ্য সিলিকন ভ্যালীতে অবস্থিত।} & \textbengali{ক্যালির্ফোনিয়ার মধ্য সিলিকন ভ্যালীতে} \\
\hline
IndicParaphrase  & Paraphrasing  & Please provide paraphrasing of the following input Bangla text. The input will be a complex Bangla sentence, the output should be a paraphrased Bangla sentence maintaining  the original information of the input text unchanged.
Note: Please do not provide anything except the paraphrased Bangla output. [INPUT: \textbengali{এসো তো, তোমার সঙ্গে কথা আছে।]} & \textbengali{আসো না, তোমার সাথে কথা বলতে চাই।} & \textbengali{['আমার কাছে এসে কথা বল।',	'আমার কাছে এসে কথা বল।',	'যাও, গিয়ে কথা বলো।',	'আপনি আসুন, কথা বলব।',	'আসুন, কথা বলুন।',	'এসো, তোমাদের সঙ্গে আলাপ করি।']} \\
\hline
BNLI  & Natural Language Inference (NLI)  & Please determine the logical relationship between the given hypothesis and premise. The input will consist of two sentences written in the Bangla language. The first sentence represents the premise, while the second sentence represents the hypothesis.  Your task is to determine whether the hypothesis is false (contradiction), true (entailment), or inconclusive (neutral) given the premise. Please output a number indicating the logical relationship between them: 0 for false (contradiction), true (entailment), and 2 for inconclusive (neutral) for neutrality. 
Note: Please avoid providing any additional information beyond the logical relationship. [PREMISE: \textbengali{আর আমি ভেবেছিলাম এটা একটা বিশেষ সুযোগ, আর এখনো, এটা এখনো, আমি মাত্র নয়টা দুই-দুই এক্স-ও যেটা আমার এএফএফসি বিমান বাহিনীর ক্যারিয়ার ক্ষেত্র ছিল।]} [HYPOTHESIS: \textbengali{আমি জানতাম না যে, সেই দিন আমিই একমাত্র ব্যক্তি ছিলাম না, যিনি ক্ষেত্রে উপস্থিত ছিলেন।]} &  0 & 2 \\
\hline
Soham News Article Classification & Text Classification  & For the Bangla news article given in the input, identify the appropriate section
title for the article. Note: Do not output any unnecessary words other than
just the section title. The response should be in English language and should
be one word. [INPUT: \textbengali{পতাকা রয়েছে যথাস্থানেই। তার সামনে জাপানের প্রধানমন্ত্রী শিনজো আবে-র সঙ্গে হাসি-হাসি মুখে করমর্দনরত নরেন্দ্র মোদী। সব কিছুই প্রথামাফিক, মাপসই, যথাযথ। মালয়েশিয়ার রাজধানী কুয়ালালামপুরে চলছে ত্রয়োদশ আসিয়ান-ইন্ডিয়া শীর্ষসম্মেলন। তার সমান্তরাল এক দ্বিপাক্ষিক বৈঠকে মিলিত হয়েছিলেন ভারত ও জাপানের প্রধানমন্ত্রীদ্বয়। সেখানেই ঘটেছে এই পতাকা-বিপর্যয়। ভারতের জাতীয় পতাকার সবুজ আংশটিকে উপরে রেখে স্থাপন করা হয়েছিল এই পতাকা। কেন এমন হল— উত্তরে সংশ্লিষ্ট ভারপ্রাপ্তরা সংবাদ সংস্থাকে জানিয়েছেন, এটা একেবারেই অনিচ্ছাকৃত ত্রুটি। সেই সঙ্গে এ-ও জানিয়েছেন, কোনও মতেই যেন নাম প্রকাশ না-পায় ভারপ্রাপ্তদের।]} & Politics & International \\
\hline
IndicSentiment & Sentiment Classification & For the given Input, is the sentiment in the input positive or negative? Note:
Please do not output anything other than the sentiment. Exclude any word
like, Sentiment in the response. [INPUT: \textbengali{এই বডি ওয়াশ খুব ভালোভাবে পরিষ্কার করে এবং ত্বক শুষ্ক হয় না।]} & Negative & Positive \\
\hline
SentNoB & Sentiment Analysis & For the given Input, is the sentiment in the input positive or negative or
neutral? Note: Please do not output anything other than the sentiment.
Exclude any word like, Sentiment in the response. 
[INPUT: \textbengali{শেষ ভিডিওটা পুরো ভুরিভোজ এর পর মিষ্টি দই এর মত লাগলো । আপনাকে সহস্র প্রণাম আদনান ভাই । দুঃখ লাগে এই ভেবে যে কেন বাংলা ভাগ হলো । আবার আসবেন কলকাতায় কিন্তু সঙ্গে বৌদিকে নিয়েএবারের মতো চাপে পড়ে নয় কিন্তু]} & Neutral & Positive \\
\hline
\end{tabular}
\caption{
Sample prompts with GPT-3.5 generated responses for Text Summarization, Question Answering, Paraphrasing, Natural Language Inference, Text Classification, and Sentiment Analysis Tasks.
}
\label{tab:sample_prompts}
\end{table*}
%%%%%%%%%%%%%%%%%%%%%%%%%%%%%%%%%%%%%%%%%%%%%%%%%%%%%%%%%%%

%%%%%%%%%%%%%%%%%%%%%%%%%%%%%%%%%%%%%%%%%%%%%%%%%%%%%%%%%%%%
\begin{table*}[htbp!]
\centering
\scriptsize
\begin{tabular}{{p{.05\linewidth}p{.10\linewidth}p{.50\linewidth}p{.14\linewidth}p{.10\linewidth}}}
\hline
\textbf{Example} & \textbf{Dataset} & \textbf{Prompt} & \textbf{GPT-3.5 Response} & \textbf{Gold Label}\\
\hline
\textbf{1} & IndicSentiment & For the given Input, is the sentiment in the input positive or negative or
neutral? Note: Please do not output anything other than the sentiment.
Exclude any word like, Sentiment in the response. 
[INPUT: \textbengali{আমি ব্যক্তিগতভাবে দেখেছি যে, গানের কথাগুলি অতিরঞ্জিত, এমনকি চলচ্চিত্রটি দেখার সময়ও আমার মনে হয়েছিল যে, আমি সেগুলিকে এগিয়ে নিয়ে যাব।} Translation: I personally found the lyrics to be exaggerated, even while watching the film I felt like I was going to take them on.] & Negative & Positive \\
\hline
\textbf{2} & IndicSentiment & For the given Input, is the sentiment in the input positive or negative or
neutral? Note: Please do not output anything other than the sentiment.
Exclude any word like, Sentiment in the response. 
[INPUT: \textbengali{বিয়ারের জন্য মরতে হবে এবং ভ্যালেট পার্কিংয়ের সুবিধাও রয়েছে।} Translation: The beer is to die for and there is also valet parking.] & Negative & Positive \\
\hline
\textbf{3} & IndicSentiment & For the given Input, is the sentiment in the input positive or negative or
neutral? Note: Please do not output anything other than the sentiment.
Exclude any word like, Sentiment in the response. 
[INPUT: \textbengali{এখানে বিভিন্ন ধরনের সেটিংস, যন্ত্রপাতি এবং অপশন রয়েছে, যার মধ্যে রয়েছে বিল্ট ইন লেসন।} Translation: There are a variety of settings, tools and options, including built-in lessons.] & Negative & Positive \\
\hline
\textbf{4} & IndicSentiment & For the given Input, is the sentiment in the input positive or negative or
neutral? Note: Please do not output anything other than the sentiment.
Exclude any word like, Sentiment in the response. 
[INPUT: \textbengali{বেশ কয়েকটি চরিত্র থাকা সত্ত্বেও বইটির সঙ্গে আমার যোগাযোগ বিচ্ছিন্ন হয়নি।} Translation: 
Despite several characters, I never lost touch with the book.] & Negative & Positive \\
\hline
\textbf{5} & IndicSentiment & For the given Input, is the sentiment in the input positive or negative or
neutral? Note: Please do not output anything other than the sentiment.
Exclude any word like, Sentiment in the response. 
[INPUT: \textbengali{ব্যবহৃত উপাদান পুরু এবং পকেটে বাইরে থেকে নিওপ্রিন আস্তরণ থাকে যা লেন্সকে বাম্প থেকে রক্ষা করে এবং হুক উপস্থিত থাকে।} Translation: 
The material used is thick and the pocket has a neoprene lining on the outside to protect the lens from bumps and hooks are present.] & Neutral & Positive \\
\hline
\textbf{6} & IndicSentiment & For the given Input, is the sentiment in the input positive or negative or
neutral? Note: Please do not output anything other than the sentiment.
Exclude any word like, Sentiment in the response. 
[INPUT: \textbengali{স্ট্যান্ড-এ রয়েছে লেভেল ইন্ডিকেটর যা বিল্ট-ইন বাবল ভিউ লেভেল এবং থ্রি-ওয়ে হেড যা ৩৬০ ডিগ্রি ঘোরানো যায়।} Translation: 
The stand has a level indicator with a built-in bubble view level and a three-way head that can be rotated 360 degrees.] & Neutral & Positive \\
\hline
\textbf{7} & IndicSentiment & For the given Input, is the sentiment in the input positive or negative or
neutral? Note: Please do not output anything other than the sentiment.
Exclude any word like, Sentiment in the response. 
[INPUT: \textbengali{ওরিয়েন্টের টাওয়ার এয়ার কুলারের ট্যাঙ্ক ক্ষমতা ১২ লিটার। এটি রিফিলিং ছাড়াই ২-৩ দিন চলে, যা ছোট আকারের কূলারের জন্য প্রত্যাশিত নয়।} Translation: 
Orient's tower air cooler has a tank capacity of 12 liters. It lasts for 2-3 days without refilling, which is not expected for a small sized cooler.] & Positive & Negative \\
\hline
\textbf{8} & SentNoB & For the given Input, is the sentiment in the input positive or negative or
neutral? Note: Please do not output anything other than the sentiment.
Exclude any word like, Sentiment in the response. 
[INPUT: \textbengali{অমায়িক ব্যবহার এই রেস্টুরেন্টের স্টাফদের।} Translation: The staff of this restaurant are accommodating.] & Neutral & Positive \\
\hline
\textbf{9} & SentNoB & For the given Input, is the sentiment in the input positive or negative or
neutral? Note: Please do not output anything other than the sentiment.
Exclude any word like, Sentiment in the response. 
[INPUT: \textbengali{রুটিওয়ালাকে অতিসত্বর বাংলাদেশ দলে তামিমের জায়গায় নেওয়া হোক । তাহলে আর ক্যাচ মিস হবেনা।} Translation: Rutiwala should be replaced by Tamim in the Bangladesh team as soon as possible. Then the catch will not be missed.] & Positive & Negative \\
\hline
\textbf{10} & SentNoB & For the given Input, is the sentiment in the input positive or negative or
neutral? Note: Please do not output anything other than the sentiment.
Exclude any word like, Sentiment in the response. 
[INPUT: \textbengali{কে বলেছে আপনাকে এখানে কেবন ব্ল্যাক কফি পাওয়া যায় ? ভালো করে জেনে তারপর ভিডিও বানান।} Translation: Who told you Kebon black coffee is available here? Know better then make videos.] & Neutral & Negative \\
\hline
\textbf{11} & SentNoB & For the given Input, is the sentiment in the input positive or negative or
neutral? Note: Please do not output anything other than the sentiment.
Exclude any word like, Sentiment in the response. 
[INPUT: \textbengali{ন থাক আপনে যান আমার এক্সাম আসে।} Translation: No you go. I have examination.] & Negative & Neutral \\
\hline
\textbf{12} & SentNoB & For the given Input, is the sentiment in the input positive or negative or
neutral? Note: Please do not output anything other than the sentiment.
Exclude any word like, Sentiment in the response. 
[INPUT: \textbengali{যারা মোবাইল দিয়ে প্রতিদিন ৪০০ থেকে ৫০০ টাকা ইনকাম করতে চান তারা আমার চেনেলটা সাবস্ক্রাইব করেন।} Translation: Those who want to earn 400 to 500 taka per day with mobile subscribe my channel.] & Positive & Neutral \\
\hline
\textbf{13} & SentNoB & For the given Input, is the sentiment in the input positive or negative or
neutral? Note: Please do not output anything other than the sentiment.
Exclude any word like, Sentiment in the response. 
[INPUT: \textbengali{আপসহীন রিপটিং এভানেই আপসহীন ভাবে খবর প্রচার করে জান।} Translation: Uncompromising reporting Know how to report news without compromise.] & Negative & Positive \\
\hline
\textbf{14} & SentNoB & For the given Input, is the sentiment in the input positive or negative or
neutral? Note: Please do not output anything other than the sentiment.
Exclude any word like, Sentiment in the response. 
[INPUT: \textbengali{এটাই ত চাই । সবাই মিলেমিশে থাকা । কিছু কিছু ইউটিউবাররা ত একজন আরেকজনের পিছনে সারাদিন গুতোগুতি করে।} Translation: That's what I want. Everyone together. Some YouTubers gossip about each other all day long.] & Neutral & Positive \\
\hline
\end{tabular}
\caption{
Error analysis of the Sentiment Analysis Task (IndicSentiment and SentNoB dataset). \textbf{Note:} The translation was not provided in the prompt. It is just included in the table for general understanding purposes.
}
\label{tab:Sentiment_error}
\end{table*}
